# Supplementary material for: Greedy-Step Off-Policy Reinforcement Learning
Source: arXiv:2102.11717 source file (2021-12-15)
Supplement: Supplementary file 1 [file appendix.pdf]

# APPENDIX

## A Method

### A.1 Algorithms

#### A.1.1 Greedy-Step Q learning

The Greedy-Step Q learning algorithm is presented in Algorithm 1.

#### A.1.2 Greedy-Step DQN

The Greedy-Step DQN algorithm is presented in Algorithm 2.

#### A.1.3 Accelerated Greedy-Step DQN

The main idea for acceleration is that the greedy-step return at timestep $t$ can be fast computed based on that at timestep $t+1$. Formally, for infinite trajectory with $N = \infty$, we have

$$\max_{1 \le n \le \infty} R_n^Q(\tau_{s_t,a_t}) = r_t + \gamma \max \left\{ \max_{a'_{t+1}} Q(s_{t+1}, a'_{t+1}), \max_{1 \le n \le \infty} R_n^Q(\tau_{s_{t+1},a_{t+1}}) \right\} \tag{1}$$

For finite trajectory with $N = T - t$ (where $T$ is the length of trajectory, $t$ is the timestep of the sample) , we have

$$\max_{1 \le n \le T-t} R_n^Q(\tau_{s_t,a_t}) = r_t + \gamma \max \left\{ \max_{a'_{t+1}} Q(s_{t+1}, a'_{t+1}), \max_{1 \le n \le T-(t+1)} R_n^Q(\tau_{s_{t+1},a_{t+1}}) \right\} \tag{2}$$

*Proof:*

Note that

$$\begin{aligned}
& R_n^Q(\tau_{s_t,a_t}) \\
&= \sum_{n'=0}^{n-1} \gamma^{n'} r_{t+n'} + \gamma^n \max_{a'_{t+n}} Q(s_{t+n}, a'_{t+n}) \\
&= r_t + \gamma \left( \sum_{n'=0}^{n-2} \gamma^{n'} r_{t+1+n'} + \gamma^{n-1} \max_{a'_{t+1+n-1}} Q(s_{t+1+n-1}, a'_{t+1+n-1}) \right) \\
&= r_t + \gamma R_{n-1}^Q(\tau_{s_{t+1},a_{t+1}})
\end{aligned}$$

**Algorithm 1** Greedy-Step Q learning

**Input:** Step $N$; Max iteration $I$,$J$.
**Initialize:** Replay buffer $\mathcal{D} = \{(s, a, \mathcal{D}_{s,a})\}_{s\in\mathcal{S},a\in\mathcal{A}}$, $\mathcal{D}_{s,a} = \emptyset$ for all $s, a$; Value function $Q_0 \in \mathbb{R}^{|\mathcal{S}|\times|\mathcal{A}|}$; $k = 0$.
**for** $i = 1, \cdots, I$ **do**
  Execute $\epsilon$-greedy policy of $Q_k$ until termination and obtain a trajectory $\tau = (s_0, a_0, r_0, s_1, a_1, r_1, \cdots, s_T)$
  **for** $t = 0, 1, \cdots, T-1$ **do**
    Store the tuple $(s_t, a_t, \tau_{s_t,a_t})$ in $\mathcal{D}_{s_t,a_t}$, where
      $\tau_{s_t,a_t} = (r_t, s_{t+1}, a_{t+1}, r_{t+1}, s_{t+2}, a_{t+2}, \cdots, s_T)$
  **end for**
  **for** $j = 1, \cdots, J$ **do**
    Sample a non-empty $\mathcal{D}_{s_t,a_t}$ from $\mathcal{D}$.
    Update the value function by the following rule

$$Q_{k+1}(s_t, a_t) = \max_{\tau_{s_t,a_t}\in\mathcal{D}_{s_t,a_t}} \max_{1\le n\le N} \left[\sum_{i=0}^{n-1} \gamma^i r_{t+i} + \gamma^n \max_{a'_{t+n}} Q_k\left(s_n, a'_{t+n}\right)\right]$$

    $k \leftarrow k + 1$
  **end for**
**end for**

**Algorithm 2** Greedy-Step DQN

**Input:** Step $N$; Max iteration $I$; Batch size $J$; Exploration rate $\epsilon$.
**Initialize:** Replay buffer $\mathcal{D}$; Q-network $Q_\theta$ with random weights $\theta$; Target Q-network $Q_{\theta'}$ with $\theta' \leftarrow \theta$.
**for** $i = 1, \cdots, I$ **do**
  Execute $\epsilon$-greedy policy of $Q_\theta$ until termination and obtain a trajectory $\tau = (s_0, a_0, r_0, s_1, a_1, \cdots, s_T)$
  **for** $t = 0, 1, \cdots, T-1$ **do**
    Store the tuple $(s_t, a_t, \tau_{s_t,a_t})$ in $\mathcal{D}$, where
      $\tau_{s_t,a_t} = (r_t, s_{t+1}, a_{t+1}, r_{t+1}, s_{t+2}, a_{t+2}, \cdots, s_T)$
  **end for**
  Sample a random mini-batch $\{(s_t^j, a_t^j, \mathcal{D}_{s_t^j,a_t^j})\}_{j=1}^J$ from $\mathcal{D}$.
  Update $\theta$ by minimizing the following loss function:

$$L(\theta) = \widehat{\mathbb{E}}\left[Q_\theta(s_t, a_t) - \max_{\tau_{s_t,a_t}\in\mathcal{D}_{s_t,a_t}} \max_{1\le n\le N} \left(\sum_{i=0}^{n-1} \gamma^i r_{t+i} + \gamma^n \max_{a'_{t+n}} Q_k\left(s_{t+n}, a'_{t+n}\right)\right)\right]^2$$

  $\theta' \leftarrow \theta$ every $C$ timesteps
**end for**

For infinite trajectory with $N = \infty$, we have

$$\begin{aligned}
&\max_{1\le n\le\infty} R_n^Q(\tau_{s_t,a_t}) \\
&= \max\left\{R_1^Q(\tau_{s_t,a_t}), R_2^Q(\tau_{s_t,a_t}), R_3^Q(\tau_{s_t,a_t}), \cdots\right\} \\
&= \max\left\{R_1^Q(\tau_{s_t,a_t}), \max\left\{R_2^Q(\tau_{s_t,a_t}), R_3^Q(\tau_{s_t,a_t}), \cdots\right\}\right\} \\
&= r_t + \gamma \max\left\{\max_{a'_{t+1}} Q(s_{t+1}, a'_{t+1}), \max\left\{R_1^Q(\tau_{s_{t+1},a_{t+1}}), R_2^Q(\tau_{s_{t+1},a_{t+1}}), \cdots\right\}\right\} \\
&= r_t + \gamma \max\left\{\max_{a'_{t+1}} Q(s_{t+1}, a'_{t+1}), \max_{1\le n\le\infty} R_n^Q(\tau_{s_{t+1},a_{t+1}})\right\}
\end{aligned} \tag{3}$$

For finite trajectory with $N = T - t$ (where $T$ is the length of trajectory, $t$ is the timestep of the sample)

$$
\begin{aligned}
&\max_{1\le n\le T-t} R_n^Q(\tau_{s_t,a_t})\\
&= \max\left\{R_1^Q(\tau_{s_t,a_t}), R_2^Q(\tau_{s_t,a_t}), R_3^Q(\tau_{s_t,a_t}), \cdots, R_{T-t}^Q(\tau_{s_t,a_t})\right\}\\
&= \max\left\{R_1^Q(\tau_{s_t,a_t}), \max\left\{R_2^Q(\tau_{s_t,a_t}), R_3^Q(\tau_{s_t,a_t}), \cdots, R_{T-t}^Q(\tau_{s_t,a_t})\right\}\right\}\\
&= r_t + \gamma \max\left\{\max_{a'_{t+1}} Q(s_{t+1}, a'_{t+1}), \max\left\{R_1^Q(\tau_{s_{t+1},a_{t+1}}), R_2^Q(\tau_{s_{t+1},a_{t+1}}), \cdots, R_{T-(t+1)}^Q(\tau_{s_{t+1},a_{t+1}})\right\}\right\}\\
&= r_t + \gamma \max\left\{\max_{a'_{t+1}} Q(s_{t+1}, a'_{t+1}), \max_{1\le n\le T-(t+1)} R_n^Q(\tau_{s_{t+1},a_{t+1}})\right\}
\end{aligned}
$$

$\square$
